# Supplementary material for: Spatial Pricing of Ride-sourcing Services in a CongestedTransportation Network
Source: arXiv:2006.00164 source file (2020-05-30)
Supplement: Supplementary file 2 [file app_data.tex]

% jd 2015-05-22 23:30
\section{Data inputs}\label{App:data_inputs}

\begin{table}[htbp]
  \centering
  \caption{Base Case Link Capacity $c_a$ (veh/h) and Free-flow Travel Time, FTT $t_a^0$ (min)}
  \resizebox{\columnwidth}{!}{
    \begin{tabular}{ccccccccccccccc}
    \toprule
    Link  & FFT   & Capacity  & \multicolumn{1}{c}{Link} & \multicolumn{1}{c}{FFT} & \multicolumn{1}{c}{Capacity } & \multicolumn{1}{c}{Link} & \multicolumn{1}{c}{FFT} & \multicolumn{1}{c}{Capacity } & \multicolumn{1}{c}{Link} & \multicolumn{1}{c}{FFT} & \multicolumn{1}{c}{Capacity } & \multicolumn{1}{c}{Link} & \multicolumn{1}{c}{FFT} & \multicolumn{1}{c}{Capacity } \\
    \midrule
1 & 12 & 777 & 17 & 6 & 235 & 32 & 10 & 300 & 47 & 10 & 151 & 62 & 12 & 152 \\
2 & 8 & 702 & 18 & 4 & 702 & 33 & 12 & 147 & 48 & 8 & 146 & 63 & 10 & 152 \\
3 & 12 & 777 & 19 & 4 & 147 & 34 & 8 & 146 & 49 & 4 & 157 & 64 & 12 & 152 \\
4 & 10 & 149 & 20 & 6 & 235 & 35 & 8 & 702 & 50 & 6 & 590 & 65 & 4 & 157 \\
5 & 8 & 702 & 21 & 20 & 151 & 36 & 12 & 147 & 51 & 16 & 150 & 66 & 6 & 146 \\
6 & 8 & 513 & 22 & 10 & 151 & 37 & 6 & 777 & 52 & 4 & 157 & 67 & 6 & 288 \\
7 & 8 & 702 & 23 & 10 & 300 & 38 & 6 & 777 & 53 & 4 & 145 & 68 & 10 & 152 \\
8 & 8 & 513 & 24 & 20 & 151 & 39 & 8 & 153 & 54 & 4 & 702 & 69 & 4 & 157 \\
9 & 4 & 533 & 25 & 6 & 417 & 40 & 8 & 146 & 55 & 6 & 590 & 70 & 8 & 150 \\
10 & 12 & 147 & 26 & 6 & 417 & 41 & 10 & 154 & 56 & 8 & 702 & 71 & 8 & 148 \\
11 & 4 & 533 & 27 & 10 & 300 & 42 & 8 & 148 & 57 & 6 & 437 & 72 & 8 & 150 \\
12 & 8 & 148 & 28 & 12 & 405 & 43 & 12 & 405 & 58 & 4 & 145 & 73 & 4 & 152 \\
13 & 10 & 300 & 29 & 8 & 146 & 44 & 10 & 154 & 59 & 8 & 150 & 74 & 8 & 153 \\
14 & 10 & 149 & 30 & 16 & 150 & 45 & 6 & 437 & 60 & 8 & 702 & 75 & 6 & 146 \\
15 & 8 & 148 & 31 & 12 & 147 & 46 & 6 & 288 & 61 & 8 & 150 & 76 & 4 & 152 \\
16 & 4 & 147 \\
    \bottomrule
    \end{tabular}%
    }
  \label{tab:capa_fft_base}%
\end{table}%
